# Supplementary material for: Weak Cube R-CNN: Weakly Supervised 3D Detection using only 2D Bounding Boxes
Source: arXiv:2504.13297 source file (2025-04-17)
Supplement: Supplementary file 1 [file X_suppl.tex]

\clearpage
\setcounter{page}{1}
\maketitlesupplementary

\section{Qualitative illustration of no rotation}
